# Supplementary material for: CO Tip Functionalization Inverts Atomic Force Microscopy Contrast via Short-Range Electrostatic Forces
Source: arXiv:1402.5246 source file (2014-02-21)
Supplement: Supplementary file 1 [file Supplemental_Information.pdf]

# Supplemental Information

## CO Tip Functionalization Inverts Atomic Force Microscopy Contrast via Short-Range Electrostatic Forces

Maximilian Schneiderbauer, Matthias Emmrich, Alfred J. Weymouth and Franz J. Giessibl

Institute of Experimental and Applied Physics, University of Regensburg, 93040 Regensburg, Germany

## S 1 Error in the calculated tip-sample distance for metal tips

According to the metal point-contact model described in the main text as well as in Ref. [1], the tunneling current is assumed to flow only between two atoms. In reality not only the front most tip atom contributes to the measured tunneling current, but also second layer atoms. The error, made by assuming that only the front most tip atom carries all current, can be estimated by comparing the two cases in Fig. S 1.

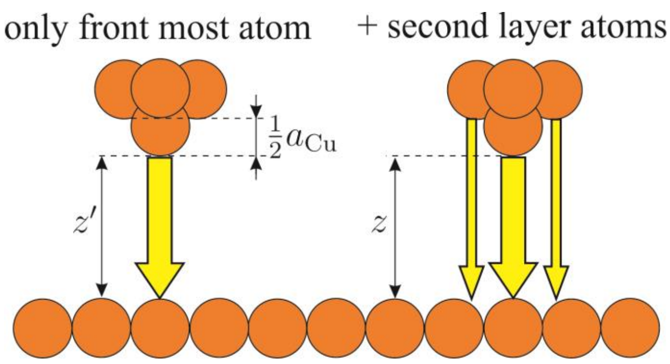


**FIG. S 1: Ideal Cu-tip pointing into <100> direction, including four second layer atoms. Left: Only the front most atom contributes to the tunneling current. Right: The four second layer atoms also contribute.**

Both tips in Fig. S 1 are at the same height above the sample, but the tunneling current measured in the right case is larger (as four second layer atoms also contribute). Now if we assume that both tips carry the same current but are at different heights *z'* and *z*, then we can calculate the apparent distance difference. For an ideal Cu tip pointing into the <100> direction the four second layer atoms are $\frac{a}{2}$ behind the front most tip atom (Cu: $a = 361$ pm). The tunneling current is given by $I(z) = I_0 e^{-2\kappa z}$ with $\kappa \approx 10^{10}\mathrm{m}^{-1}$ and we can write:

$$I_{left}(z') = I_{right}(z)$$

$$I_0 \cdot e^{-2\kappa z'} = I_0 \cdot e^{-2\kappa z} + 4 \cdot I_0 e^{-2\kappa\left(z+\frac{a}{2}\right)}$$

$$\Rightarrow z - z' = 50.6 \text{ pm}$$

The tip-sample distance $z_{s-s}$, defined in the main text, is therefore only a lower boundary, whereby the real distance should at least be 50 pm larger.

## S 2 Determination of the tip-sample distance for CO terminated tips

To calculate the tip-sample distance for a CO terminated tip, one has to determine the point conductance of a CO molecule on a metal surface, here Cu(100). Therefore, we performed the experiment, schematically described in Fig. S 2(a). We recorded an $I_{Cu}(z)$ spectra with a Cu terminated tip over Cu(100), right after we picked up a CO molecule, which was laying close by, and recorded another $I_{CO}(z)$ spectra. Both spectra were recorded within one minute and the *z*-range of the scanning piezo $z_{piezo}$ overlapped. In Fig. S 2(b) the corresponding conductance spectra normalized to metal point-contact are shown, for Cu (black) and CO (red) tip, where the abscissa is the absolute piezo-range $z_{piezo}$. For a certain value of $z_{piezo}$ in the $I_{Cu}(z)$ spectra, the tip-sample distance after picking up a CO is reduced by the length extension of the CO molecule $l_{CO}$, see Fig. S 2(a). Hence, the $I_{CO}(z)$ spectra has to be shifted towards the sample by $l_{CO}$, as depicted in Fig. S 2(b). We estimated $l_{CO}$ by adding the CO's binding length of 115 pm with the atomic radii of C (70 pm) and O (60 pm). Not to underestimate the tip-sample distance we took $l_{CO} = 250$ pm and to estimate a lower boundary here as well. In Fig. S 2(c) we fitted the normalized conductance of the Cu terminated tip with an exponential function and extrapolated the curve up to ${}^{G}/_{G_0} = 1$ and defined a new abscissa with $z_{s-s} = 0$ at this point. The shifted conductance for the CO terminated tip was also normalized to the metal point-contact conductance of $G_0 = (12906\ \Omega)^{-1}$. Its exponential fit (red curve in Fig. S 2(c)) intersects the ordinate at 0.03191 resulting in a point conductance of $G_0(CO) = (404497\ \Omega)^{-1}$ for the CO terminated tip. Taking into account the error made within the metal point-contact model (see S 1) and the estimated length of the CO molecule $l_{CO}$ the calculated tip-sample distance $z_{s-s}$ using $G_0(CO)$ is an underestimate of at least 55 pm.

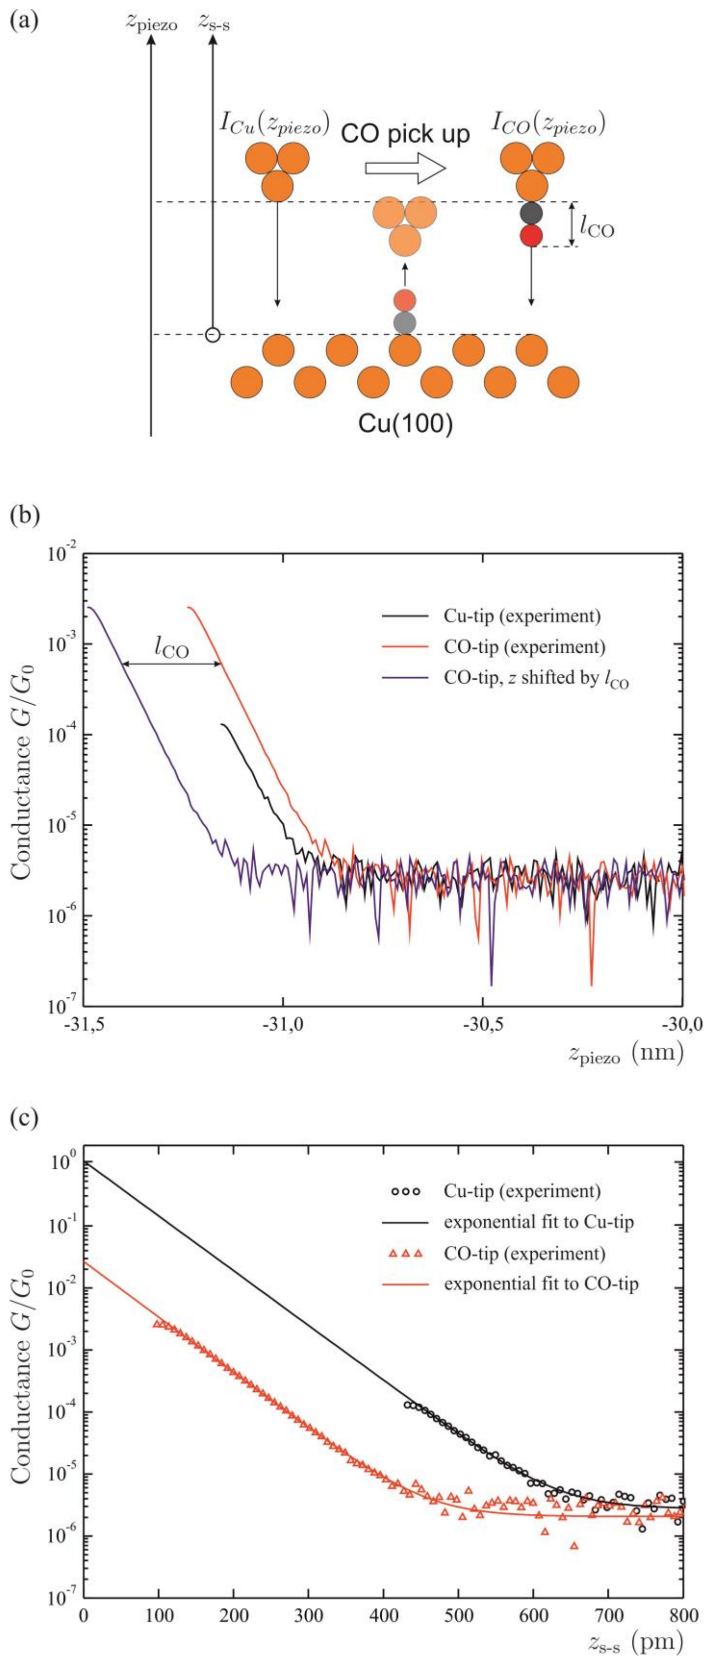


**FIG. S 2: (a) Schematic of the experiment to determine the point contact of a CO terminated tip. (b) Conductance in unites of the quantum conductance versus distance curve for Cu (black) and CO (red) tip. In addition the shifted CO curve is shown (blue). (c) Extrapolated conductance curves, where for Cu tip $G(z = 0) = G_0$ holds. The intersection of the shifted CO curve with the ordinate gives the point conductance of the CO terminated tip on a metallic sample.**

## S 3 Electrostatic simulation

The electric field outside a certain radial charge distribution can be seen as originating from a point charge centered in the volume. Therefore, the charges of the sample atoms were fixed on their atomic core positions. The z-component of the electrostatic field arising from 7x7 $Cu_2N$ unit cells was numerically calculated by:

$$E_z(\boldsymbol{r}) = \frac{1}{4\,\pi\varepsilon_0}\left[\sum_{N\,sites}(-1.2e)\frac{\boldsymbol{r}-\boldsymbol{r}_N}{|\boldsymbol{r}-\boldsymbol{r}_N|^3}\cdot\begin{pmatrix}0\\0\\1\end{pmatrix} + \sum_{\substack{surface\,Cu\\sites}}(+0.5e)\frac{\boldsymbol{r}-\boldsymbol{r}_{s-Cu}}{|\boldsymbol{r}-\boldsymbol{r}_{s-Cu}|^3}\cdot\begin{pmatrix}0\\0\\1\end{pmatrix} + \sum_{\substack{subsurface\\Cu\,sites}}(+0.1e)\frac{\boldsymbol{r}-\boldsymbol{r}_{ss-Cu}}{|\boldsymbol{r}-\boldsymbol{r}_{ss-Cu}|^3}\cdot\begin{pmatrix}0\\0\\1\end{pmatrix}\right] \quad .$$

The electrostatic force on the tip dipole $p = q\cdot d$ (q: dipole charge, d: dipole distance) was calculated by:

$$F_z(x,y,z_{c-c}) = \pm q\cdot E_z(x,y,z_{c-c}) \pm q\cdot E_z(x,y,z_{c-c}+d) \quad .$$

For the Cu terminated tip $q = \pm 0.13e$, $d = r_{Cu} = 135$ pm and $z_{c-c} = z_{s-s} + 2\cdot r_{Cu}$. For the CO terminated tip $q = \pm 0.03e$, $d = l_{CO} = 115$ pm and $z_{c-c} = z_{s-s} + r_{Cu} + r_O$. See also Fig. S 3.

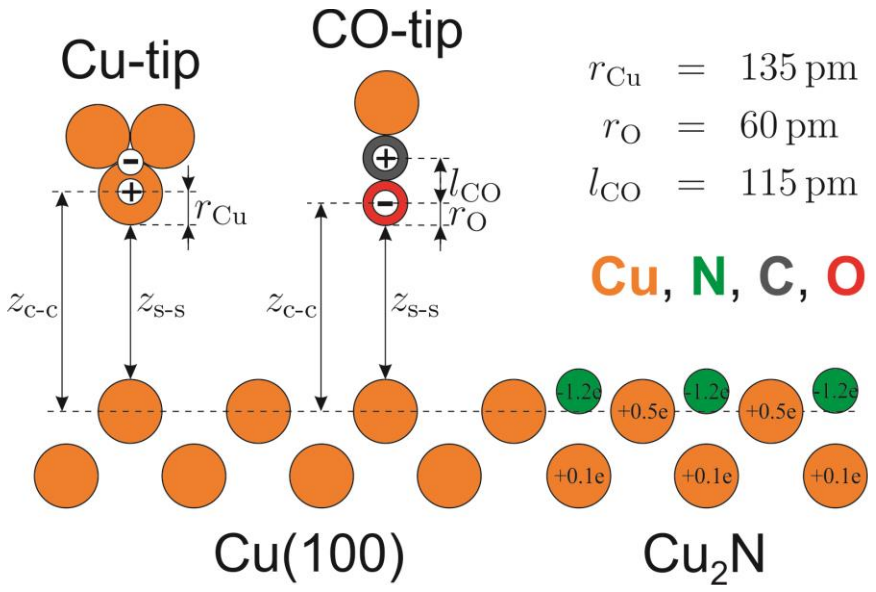


**FIG. S 3: Deducing the core-core distance $z_{c-c}$ from the experimental shell-shell distance $z_{s-s}$ for both tip terminations.**

## References:


[1] M. Ternes, C. P. Lutz, C. F. Hirjibehedin, F. J. Giessibl, and A. J. Heinrich, Science **319**, 1066 (2008).
